# Supplementary material for: Magnetic quenching of the inverse cascade in rapidly rotating convective turbulence
Source: arXiv:1807.03268 ancillary file (2019-03-12)
Supplement: Supplementary file 1 [file Maffei_et_al_PRF_supplementary.pdf]

# Supplementary online material to the article "Magnetic quenching of the inverse cascade in rapidly rotating convective turbulence"

Stefano Maffei,[1] Michael A. Calkins,[1] Keith Julien,[2] and Philippe D. Marti[3,4]

[1]*Department of Physics, University of Colorado, Boulder, Colorado 80309, USA*

[2]*Department of Applied Mathematics, University of Colorado, Boulder, Colorado 80309, USA*

[3]*Center for Climate System Modeling, ETH Zürich, CH-8092, Switzerland*

[4]*Department of Earth Sciences, ETH Zürich, CH-8092, Switzerland*

| $\widetilde{Ra}$ | $\widetilde{Q}$ | $\widetilde{k}_c$ | $N_x$ | $N_Z$ | $\Delta t$ | $\widetilde{Re}$ | $\widetilde{N}$ |
|---|---|---|---|---|---|---|---|
| 20 | 0 | 1.3048 | 128 | 64 | $5\times10^{-2}$ | $3.563\pm0.101$ | - |
| 20 | 0.05 | 1.2883 | 192 | 96 | $2\times10^{-2}$ | $3.5807\pm0.0956$ | $(1.3964\pm0.0373)\times10^{-2}$ |
| 20 | 0.1 | 1.2797 | 128 | 64 | $1\times10^{-2}$ | $3.564\pm0.101$ | $(2.8058\pm0.0795)\times10^{-2}$ |
| 20 | 0.2 | 1.2545 | 192 | 96 | $2\times10^{-2}$ | $3.657\pm0.114$ | $(5.469\pm0.171)\times10^{-2}$ |
| 20 | 0.5 | 1.1710 | 192 | 96 | $2\times10^{-2}$ | $3.7501\pm0.0907$ | $(1.3333\pm0.0322)\times10^{-1}$ |
| 20 | 1 | 1.0158 | 192 | 96 | $2\times10^{-2}$ | $3.936\pm0.105$ | $(2.5407\pm0.0678)\times10^{-1}$ |
| 20 | 2 | 0.5858 | 128 | 64 | $1\times10^{-2}$ | $4.2765\pm0.0821$ | $(4.6767\pm0.0898)\times10^{-1}$ |
| 40 | 0 | 1.3048 | 192 | 96 | $5\times10^{-4}$ | $10.652\pm0.303$ | - |
| 40 | 0.05 | 1.2883 | 192 | 96 | $1\times10^{-3}$ | $10.663\pm0.258$ | $(4.689\pm0.113)\times10^{-3}$ |
| 40 | 0.1 | 1.2797 | 192 | 96 | $1\times10^{-3}$ | $10.533\pm0.275$ | $(9.494\pm0.248)\times10^{-3}$ |
| 40 | 0.2 | 1.2545 | 192 | 96 | $1\times10^{-3}$ | $10.487\pm0.306$ | $(1.9071\pm0.0556)\times10^{-2}$ |
| 40 | 0.5 | 1.1710 | 192 | 96 | $1\times10^{-3}$ | $10.559\pm0.282$ | $(4.735\pm0.126)\times10^{-2}$ |
| 40 | 1 | 1.0158 | 192 | 96 | $5\times10^{-4}$ | $10.897\pm0.270$ | $(9.177\pm0.227)\times10^{-2}$ |
| 40 | 2 | 0.5858 | 192 | 96 | $1\times10^{-3}$ | $11.497\pm0.251$ | $(1.7396\pm0.0380)\times10^{-1}$ |
| 80 | 0 | 1.3048 | 256 | 128 | $1\times10^{-6}$ | $22.382\pm0.610$ | - |
| 80 | 0.1 | 1.2797 | 256 | 128 | $3\times10^{-4}$ | $22.000\pm0.575$ | $(4.545\pm0.119)\times10^{-3}$ |
| 80 | 0.2 | 1.2545 | 256 | 128 | $3\times10^{-4}$ | $21.397\pm0.448$ | $(9.347\pm0.196)\times10^{-3}$ |
| 80 | 0.5 | 1.1710 | 256 | 128 | $7\times10^{-4}$ | $20.368\pm0.330$ | $(2.4548\pm0.0398)\times10^{-2}$ |
| 80 | 1 | 1.0158 | 256 | 128 | $3\times10^{-4}$ | $19.569\pm0.432$ | $(5.110\pm0.113)\times10^{-2}$ |
| 80 | 2 | 0.5858 | 256 | 128 | $3\times10^{-4}$ | $19.119\pm0.114$ | $(1.04608\pm0.00624)\times10^{-1}$ |
| 120 | 0 | 1.3048 | 256 | 256 | $1\times10^{-4}$ | $38.41\pm2.31$ | - |
| 120 | 0.1 | 1.2797 | 256 | 256 | $1\times10^{-4}$ | $33.26\pm1.08$ | $(3.0066\pm0.0976)\times10^{-3}$ |
| 160 | 0 | 1.3048 | 256 | 256 | $1\times10^{-4}$ | $51.86\pm3.68$ | - |
| 160 | 0.1 | 1.2797 | 256 | 256 | $3\times10^{-4}$ | $50.50\pm2.02$ | $(1.9802\pm0.0792)\times10^{-3}$ |
| 160 | 0.2 | 1.2545 | 256 | 256 | $1\times10^{-4}$ | $49.16\pm2.41$ | $(4.068\pm0.199)\times10^{-3}$ |
| 160 | 0.5 | 1.1710 | 256 | 256 | $1\times10^{-4}$ | $44.59\pm1.13$ | $(1.1213\pm0.0284)\times10^{-2}$ |
| 160 | 1 | 1.0158 | 256 | 256 | $1\times10^{-4}$ | $41.50\pm1.30$ | $(2.4096\pm0.0755)\times10^{-2}$ |
| 160 | 2 | 0.5858 | 256 | 256 | $5\times10^{-4}$ | $36.837\pm0.370$ | $(5.4293\pm0.0545)\times10^{-2}$ |
| 200 | 1 | 1.0158 | 384 | 384 | $1\times10^{-4}$ | $54.01\pm1.23$ | $(1.8515\pm0.0422)\times10^{-2}$ |

TABLE I. Details of the numerical simulations. $\widetilde{Ra} = Ra_H E_H^{4/3}$ and $\widetilde{Q} = Q_H E_H^{2/3}$ are the asymptotically scaled Rayleigh and Chandrasekhar number, respectively; $\widetilde{k}_c$ is the critical horizontal wavenumber at the onset of convection; $N_x = N_y$ is the horizontal spatial resolution (in Fourier space) and $N_Z$ is the vertical spatial resolution (in terms of Chebyshev modes); $\Delta t$ is the smallest stable time-step size used in each simulation. Both vertical and horizontal resolutions are further de-aliased using the 2/3 rule. The small-scale Reynolds number is based on the vertical (baroclinic) velocity $\widetilde{Re} = \mathrm{rms}(w)$, where $\mathrm{rms}(\cdot)$ is the rms value of the argument over the volume of integration and the interaction parameter is defined as $\widetilde{N} = \widetilde{Re}^{-1}\widetilde{Q}$. The uncertainties on $\widetilde{Re}$ are given as the standard deviations of $w$ and the ones on $\widetilde{N}$ are calculated using standard error propagation. In each case the non-dimensional horizontal box dimensions are $10\widetilde{L}_c \times 10\widetilde{L}_c$ where $\widetilde{L}_c = 2\pi/\widetilde{k}_c$ is the critical horizontal wavelength. Simulations were initialised either from random initial conditions or (especially for higher values of $\widetilde{Ra}$) from cases with either lower $\widetilde{Ra}$ or higher $\widetilde{Q}$. The general criteria was to initialise each simulation from a state devoid of LSV, so to track their growth in time.

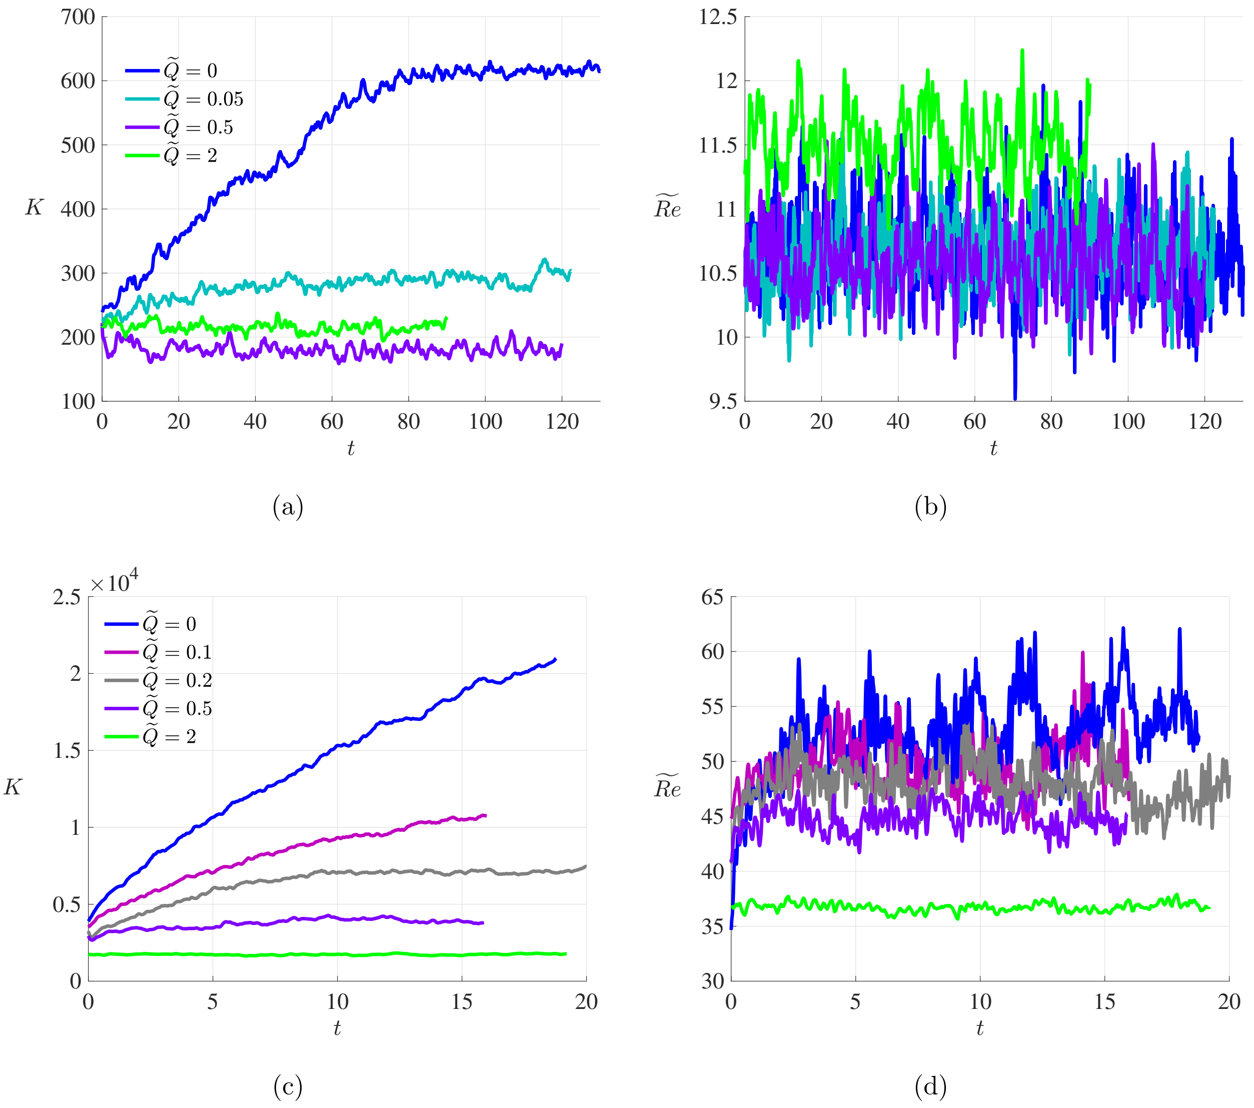


FIG. 1. Time series of the total kinetic energy per unit volume $K=(2V)^{-1}\int_V |\mathbf{u}|^2 dV$ (a), (c) and of $\widetilde{Re}=\sqrt{V^{-1}\int_V w^2 dV}$ (b), (d) for $\widetilde{Ra}=40$ (a), (b) and $\widetilde{Ra}=160$ (c), (d) and various values of $\widetilde{Q}$. Notice that as for $\widetilde{Q}\leq 0.05$ (for $\widetilde{Ra}=40$) and $\widetilde{Q}\leq 0.2$ (for $\widetilde{Ra}=160$) the formation of LSV leads to a growth of kinetic energy with time. $\widetilde{Re}$ reaches a statistically stationary value, indicating that the formation of LSV does not significantly influence the baroclinic (convective) dynamics.
